# Supplementary material for: When Life Gives You Lemons, Make Cherryade: Converting Feedback from Bad Responses into Good Labels
Source: arXiv:2210.15893 source file (2022-10-28)
Supplement: Supplementary file 1 [file A_additional_exp_results.tex]

\subsection{Additional Experimental Results}
% Quantitative Evaluation on NQ valid
\begin{table}[H]
\centering
\small
% \resizebox{\linewidth}{!}{
\begin{tabular}{lllcc}
\textbf{Response Model} & \textbf{Knowledge Model} & \textbf{Knowledge} & \textbf{AP} $\uparrow$ & \textbf{GAP} \\ 
 \hline
 \hline \\
\multicolumn{2}{l}{\textbf{Baselines}} \\ 
BART & - & - & 3.2 & -\\ 
BART RAG DPR & - & Wiki & 11.4 & - \\ 
- & T5 FID DPR & Wiki & 45.6 & - \\ 
\hline \\
\multicolumn{2}{l}{\textbf{\sss}} \\ 
% BART & RAG DPR C. & & \\ 
BART & T5 FID DPR & Wiki & 38.1 & 77.2 \\ 
BART + filter & T5 FID DPR & Wiki & 45.7 & 97.6 \\ 
\hline
BART & Oracle & Gold & 74.6 & 74.6\\ 
BART + filter & Oracle & Gold & 96.6 & 96.6\\ 
\end{tabular}
% }
\caption{Quantitative Evaluations on Natural Questions Valid.}
\label{tab:nq_quantitative_valid}
\end{table}

%% Quantitative Results LightQA Valid
\begin{table}[H]
\centering
\small
% \resizebox{\linewidth}{!}{
\begin{tabular}{llllcc}
\textbf{Response Model} & \textbf{Knowledge Model} & \textbf{RM Train Data} & \textbf{KM Train Data} & \textbf{AP} $\uparrow$ & \textbf{GAP} \\ 
 \hline
 \hline \\
\multicolumn{3}{l}{\textbf{Baselines}} \\ 
BART & - & LightWild & - & 27.5 & - \\ 
BART & - & LightQA & - & 86.1 & - \\ 
BART & - & LightWild+LightQA & - & 80.8 & - \\ 
\hline \\
\multicolumn{3}{l}{\textbf{\sss}} \\ 
BART & BART & LightWild & LightWild & 37.3 & 99.6 \\ 
BART & BART & LightWild & LightQA & \textbf{92.8} & 98.9\\ 
BART & BART & LightWild & LightWild+LightQA & 92.0 & 98.9 \\ 
BART & Oracle & LightWild & - & 99.1 & 99.1\\ 
\end{tabular}
% }
\caption{Quantitative Evaluations on LightQA Valid.}
\label{tab:sumaryqa_quantitative}
\end{table}

%% Quantitative Results light-dialog-wild Valid
\begin{table}[H]
\centering
\small
% \resizebox{\linewidth}{!}{
\begin{tabular}{llllcccc}
\textbf{Response Model} & \textbf{Knowledge Model} & \textbf{RM Train Data} & \textbf{KM Train Data} & \textbf{PPL} $\downarrow$ & \textbf{F1} $\uparrow$ & \textbf{Rare F1} $\uparrow$ & \textbf{GAP}\\
 \hline
 \hline \\

\multicolumn{2}{l}{\textbf{Baselines}} \\ 
BART & - & LightWild & - & \textbf{17.1} & 15.4 & 9.5 & - \\ 
BART & - & LightWild+LightQA & - & 17.3 & 15.8 & 9.9 & - \\ 
\hline \\
\multicolumn{2}{l}{\textbf{\sss}} \\ 
BART & BART & LightWild & LightWild & 26.2 & \textbf{16.7} & 10.7 & 99.6 \\
BART & BART & LightWild & LightWild+LightQA & 26.7 & 16.4 & 10.6 & 99.4 \\ 
BART  {\tiny (shared params)} & BART {\tiny (shared params)} & LightWild & LightWild & 27.2 & \textbf{16.7} & \textbf{10.9} & 99.8 \\ 
BART & Oracle & LightWild & - & 11.3 & 31.4 & 30.8 & 99.0 \\ 
\hline \\
\multicolumn{2}{l}{\textbf{\sss - Score Conditioned}} \\ 
BART & BART 0 & LightWild & LightWild & 18.9 & 16.3 & 10.3 & 62.2 \\
BART & BART 2 & LightWild & LightWild & 19.5 & 16.6 & 10.8 & 80.3 \\
BART & BART 6 & LightWild & LightWild & 20.6 & 16.7 & 11.0 & 94.7 \\
BART & BART 10 & LightWild & LightWild & 22.7 & 16.7 & 11.0 & 99.2\\
BART & Oracle 0 & LightWild & - & 12.6 & 27.3 & 25.6 & 80.1 \\ 
BART & Oracle 2 & LightWild & - & 12.4 & 28.4 & 27.3 & 87.4 \\ 
BART & Oracle 6 & LightWild & - & 12.1 & 29.4 & 29.0 & 93.4 \\ 
BART & Oracle 10 & LightWild & - & 12.0 & 30.4 & 30.3 & 98.5 \\ 
\end{tabular}
% }
\caption{Quantitative Evaluations on LightWild Valid.}
\label{tab:light_quantitative_valid}
\end{table}

%% WoW Quantitative Results test
\begin{table}[H]
\begin{center}
\resizebox{\linewidth}{!}{
\begin{tabular}{lll|rrrrrr|rrrrrr}
& & &\multicolumn{6}{c}{Test Random Split} & \multicolumn{6}{c}{Test Unseen Split} \\
Response Model & Knowledge Model & Knowledge & PPL & F1 & KF1 & RF1 & B4 & RL &  PPL & F1 & KF1 & RF1 & B4 & RL \\
\hline
\hline
\multicolumn{2}{l}{\textbf{Baselines}} \\ 
BART & None & None & 14.7 & 20.9 & 17.4 & 14.7 & 1.7 & 20.3 & 18.9 & 18.8 & 15.1 & 12.1 & 0.9 & 18.4 \\
% BART RAG DPR (Paper) & None & Wiki & 12.7 & 22.4 & 22.5 & & 3.4 & 22.9 & 14.5 & 21.7 & 20.8 & & 2.6 & 21.7\\
BART RAG DPR & None & Wiki & \textbf{11.5} & \textbf{22.6} & 26.1 & \textbf{17.7} & \textbf{3.7} & \textbf{23.2} & \textbf{13.1} & \textbf{21.5} & 22.7 & \textbf{16.5} & \textbf{3.0} & \textbf{21.9} \\
\hline
\multicolumn{2}{l}{\textbf{\sss}} \\ 
BART & RAG DPR & Wiki & 17.9 & 21.3 &\textbf{29.2} & \textbf{17.7} & 3.5 & 22.4 & 21.1 & 19.2 & \textbf{24.3} & 15.0 & 2.5 & 20.0\\
RAG DPR {\tiny (shared params)} & RAG DPR {\tiny (shared params)} & Wiki & 18.3 & 22.0 & 27.3 & 17.4 & \textbf{3.7} & 22.7 & 22.3 & 19.9 & 23.2 & 14.7 & 2.8 & 20.5\\
\hline
BART & Oracle & Gold & 8.1 & 37.4 & 68.6 & 39.8 & 11.1 & 39.4 & 8.62 & 37.4 & 69.1 & 39.5 & 10.9 & 39.9\\
\end{tabular}
}
\end{center}
\caption{Quantitative Evaluations on Wizard of Wikipedia Test (seen and unseen split). We compare against the ground truth dialogue response in terms of perplexity (PPL), F1, Knowledge F1 (KF1), Rare F1 (RF1), BLEU-4 (B4), and ROUGE-L (RL).}
% Note: Ablation table # 0
\label{tab:wow_quantitative_test_seen_unseen}
\end{table}

%% WoW Quantitative Results valid
\begin{table}[H]
\begin{center}
\resizebox{\linewidth}{!}{
\begin{tabular}{lll|rrrrrr|rrrrrr}
& & &\multicolumn{6}{c}{Valid Seen Split} & \multicolumn{6}{c}{Valid Unseen Split} \\
Response Model & Knowledge Model & Knowledge & PPL & F1 & KF1 & RF1 & B4 & RL &  PPL & F1 & KF1 & RF1 & B4 & RL \\
\hline
\hline
\multicolumn{2}{l}{\textbf{Baselines}} \\ 
BART & None & None & 14.8 & 20.9 & 17.6 & 14.8 & 1.7 & 20.7 & 18.7 & 19.7 & 15.5 & 13.1 & 0.9 & 19.0 \\
BART RAG DPR & None & Wiki & \textbf{11.6} & 22.6 & 26.0 & 17.9 & 3.9 & 23.6 & \textbf{13.4} & \textbf{21.7} & 22.6 & 16.8 & 2.7 & \textbf{21.7} \\
\hline
\multicolumn{2}{l}{\textbf{\sss}} \\ 
BART & RAG DPR & Wiki & 17.7 & 22.0 &\textbf{30.6} & \textbf{18.6} & \textbf{4.3} & 23.5 & 20.6 & 20.6 & \textbf{26.2} & \textbf{17.2} & \textbf{3.0} & 20.9\\
RAG DPR {\tiny (shared params)} & RAG DPR {\tiny (shared params)} & Wiki & 18.1 & \textbf{22.7} & 28.1 & 18.1 & 4.2 & \textbf{23.7} & 22.4 & 21.0 & 23.1 & 16.4 & 2.4 & 20.9\\
\hline
BART & Oracle & Gold & 8.5 & 37.0 & 68.1 & 39.2 & 10.8 & 39.3 & 8.7 & 37.2 & 69.6 & 39.6 & 10.5 & 38.6\\
\end{tabular}
}
\end{center}
\caption{Quantitative Evaluations on Wizard of Wikipedia Valid (seen and unseen split). We compare against the ground truth dialogue response in terms of perplexity (PPL), F1, Knowledge F1 (KF1), Rare F1 (RF1), BLEU-4 (B4), and ROUGE-L (RL).}
% Note: Ablation table # 0
\label{tab:wow_quantitative_valid}
\end{table}

%% WoW Quantitative Results confidence-conditioned test
\begin{table}[H]
\begin{center}
% \resizebox{\linewidth}{!}{
\small
\begin{tabular}{llll|rrrrrrr}
% & & &\multicolumn{6}{c}{WoW Test Seen} & \multicolumn{6}{c}{WoW Test Unseen} \\
Response Model & Knowledge Model & Knowledge & Confidence & PPL & F1 & KF1 & RF1 & PKF1 & B4 & RL \\
\hline
\hline
% \multicolumn{2}{l}{\textbf{Baselines}} \\ 
% BART & None & None & None & 14.7 & 20.9 & 17.4 & 14.7 & - & 1.7 & 20.3 \\
% % BART RAG DPR (Paper) & None & Wiki & 12.7 & 22.4 & 22.5 & & 3.4 & 22.9 & 14.5 & 21.7 & 20.8 & & 2.6 & 21.7\\
% BART RAG DPR & None & Wiki & None & 11.5 & 22.6 & 26.1 & 17.7 & - & 3.6 & 23.2 \\
% \hline
\multicolumn{2}{l}{\textbf{\sss}} \\ 
BART & RAG DPR & Wiki & 0 & 13.6 & 22.0 & 22.4 & 16.6 &	37.9 & 2.9 & 22.4 \\
BART & RAG DPR & Wiki & 2 & 13.6 & 22.6 & 26.4 & 17.9 & 57.0 & 3.7 & 23.4 \\
BART & RAG DPR & Wiki & 6 & 13.9 & 22.4 & 27.2 & 18.0 &	64.2 & 3.9 & 23.1 \\
BART & RAG DPR & Wiki & 10 & 14.3 &	22.2 & 27.2 & 18.0 & 66.8 &	3.8 & 22.9 \\
\hline
BART & RAG DPR & Wiki & None & 17.9 & 21.3 & 29.2 & 17.7 & 76.4 & 3.5 & 22.4 \\
\hline
BART & Oracle & Wiki & 0 & 9.2 & 26.5 & 30.3 & 22.7 & 30.3 & 5.1 & 27.0 \\
BART & Oracle & Wiki & 2 & 8.5 & 33.6 & 47.8 & 33.1 & 47.8 & 9.5 & 35.0 \\
BART & Oracle & Wiki & 6 & 8.3 & 36.8 & 56.8 & 37.6 & 56.8 & 11.1 & 38.3 \\
BART & Oracle & Wiki & 10 & 8.2 & 37.7 & 60.6 & 39.2 & 60.6 & 11.5 & 39.2 \\
\hline
BART & Oracle & Gold & None & 8.1 & 37.4 & 68.6 & 39.8 & 68.6 & 11.1 & 39.4 \\
\end{tabular}
% }
\end{center}
\caption{Quantitative Evaluations of the confidence-conditioned \sss model on Wizard of Wikipedia Test (random split). We add a fixed confidence score of \{0, 2, 6, 10\} to the input. We compare against the ground truth dialogue response in terms of perplexity (PPL), F1, Knowledge F1 (KF1), Predicted Knowledge F1 (PKF1), Rare F1 (RF1), BLEU-4 (B4), and ROUGE-L (RL). We see that with increasing confidence, the PKF1 increases which leads to an increase in KF1 and PPL.}
% Note: Ablation table # 0
\label{tab:wow_quantitative_confidence_score_test}
\end{table}

\subsection{LightWild Confidence Conditioning} \label{app:lightwild_control}
We train a BART dialogue response model based on the confidence-conditioned training strategy described in Section \ref{sec:model_k2r}. During training, we replace the correct knowledge with a random noun from the history with probability $p$ and provide $\tilde{p} = \textrm{round}(10* p)$ to the input. The model learns to scale its trust in the knowledge prediction based on the $\tilde{p}$ value in the input. In Table~\ref{tab:lightqa_confcond}, we show the results of this dialogue model when combined either with the BART knowledge model trained on LightWild+LightQA or an oracle knowledge model. For both variants, we see an apparent increase in the share of examples for which the dialogue response has the generated answer present (GAP) when increasing the confidence score. This means that we can adjust the confidence score to influence how much the dialogue model trusts the knowledge prediction. 
As observed before in the WoW results, we also see that the perplexity increases with higher confidences when using the knowledge prediction model but decreases when using the oracle. However, again, the perplexity increases don't lead to worse performance in the F1 metrics. On the contrary, a confidence score of 6, which translates to a GAP of 94.1\%, performs the best in F1 and RF1 for the non-oracle model.

%% Confidence-Score Conditioning light-dialog-wild
\begin{table}[H]
\centering
\small
%\resizebox{\linewidth}{!}{
\begin{tabular}{lc|cccc}
\textbf{Model} & \textbf{Confidence} & \textbf{PPL} $\downarrow$ & \textbf{F1} $\uparrow$ & \textbf{RF1} $\uparrow$ & \textbf{GAP}\\
 \hline
 \hline

% \multicolumn{2}{l}{\textbf{Baselines}} \\ 
% BART & - & LightWild & - & \textbf{16.8} & 15.4 & 9.5 & - \\ 
% BART & - & LightWild+LightQA & - & 17.1 & 15.5 & 9.6 & - \\ 
% \hline \\
% \multicolumn{2}{l}{\textbf{\sss}} \\ 
% BART & BART & LightWild & LightWild & 25.7 & \textbf{16.6} & \textbf{10.4} & 99.5 \\
% BART & BART & LightWild & LightWild+LightQA & 25.9 & 16.5 & 10.3 & 99.4 \\ 
% BART  (shared params) & BART (shared params) & LightWild & LightWild & 26.2 & 16.3 & 10.2 & 99.6 \\ 
% BART & Oracle & LightWild & - & 11.4 & 30.9 & 30.0 & 99.3 \\ 
% \hline \\
% \multicolumn{2}{l}{\textbf{\sss - Score Conditioned}} \\ 

\sss BART &  0 & 18.5 & 16.3 & 10.0 & 59.5 \\
(LightWild+ & 2 & 19.1 & 16.4 & 10.2 & 78.4 \\
 LightQA KM) & 6 & 20.2 & 16.4 & 10.3 & 94.1 \\
 & 10 & 22.3 & 16.2 & 10.1 & 99.0\\
 \hline
%  \\
\sss BART & 0 & 12.7 & 27.4 & 25.5 & 79.0 \\ 
  (oracle KM) & 2 & 12.4 & 28.6 & 27.5 & 86.7 \\ 
 & 6 & 12.1 & 29.9 & 29.2 & 94.2 \\ 
 & 10 & 12.0 & 30.1 & 30.0 & 98.3 \\ 
\end{tabular}
%}
\caption{Confidence-conditioned model on LightWild.}
\label{tab:lightqa_confcond}
\end{table}
